# Supplementary material for: Exploiting Facial Relationships and Feature Aggregation for Multi-Face Forgery Detection
Source: arXiv:2310.04845 source file (2023-10-07)
Supplement: Supplementary file 1 [file supplementary.tex]

%File: anonymous-submission-latex-2024.tex
% \documentclass[letterpaper]{article} % DO NOT CHANGE THIS
\usepackage[submission]{aaai24}  % DO NOT CHANGE THIS
\usepackage{times}  % DO NOT CHANGE THIS
\usepackage{helvet}  % DO NOT CHANGE THIS
\usepackage{courier}  % DO NOT CHANGE THIS
\usepackage[hyphens]{url}  % DO NOT CHANGE THIS
\usepackage{graphicx} % DO NOT CHANGE THIS
\urlstyle{rm} % DO NOT CHANGE THIS
  % DO NOT CHANGE THIS
\usepackage{natbib}  % DO NOT CHANGE THIS AND DO NOT ADD ANY OPTIONS TO IT
\usepackage{caption} % DO NOT CHANGE THIS AND DO NOT ADD ANY OPTIONS TO IT
\frenchspacing  % DO NOT CHANGE THIS
\setlength{\pdfpagewidth}{8.5in} % DO NOT CHANGE THIS
\setlength{\pdfpageheight}{11in} % DO NOT CHANGE THIS
%
% These are recommended to typeset algorithms but not required. See the subsubsection on algorithms. Remove them if you don't have algorithms in your paper.
\usepackage{algorithm}
\usepackage{algorithmic}
\usepackage{amsmath}
\usepackage{amssymb}
\usepackage{multirow}
\usepackage{booktabs}
\usepackage{amssymb}
\usepackage{graphicx} % 用于插入图片
\usepackage{subcaption} % 用于创建子图
%
% These are are recommended to typeset listings but not required. See the subsubsection on listing. Remove this block if you don't have listings in your paper.
\usepackage{newfloat}
\usepackage{listings}
\DeclareCaptionStyle{ruled}{labelfont=normalfont,labelsep=colon,strut=off} % DO NOT CHANGE THIS
\lstset{%
	basicstyle={\footnotesize\ttfamily},% footnotesize acceptable for monospace
	numbers=left,numberstyle=\footnotesize,xleftmargin=2em,% show line numbers, remove this entire line if you don't want the numbers.
	aboveskip=0pt,belowskip=0pt,%
	showstringspaces=false,tabsize=2,breaklines=true}
\floatstyle{ruled}
\newfloat{listing}{tb}{lst}{}
\floatname{listing}{Listing}
%
% Keep the \pdfinfo as shown here. There's no need
% for you to add the /Title and /Author tags.
\pdfinfo{
/TemplateVersion (2024.1)
}

% DISALLOWED PACKAGES
% \usepackage{authblk} -- This package is specifically forbidden
% \usepackage{balance} -- This package is specifically forbidden
\usepackage{color}

\setcounter{secnumdepth}{2} %May be changed to 1 or 2 if section numbers are desired.

% The file aaai24.sty is the style file for AAAI Press
% proceedings, working notes, and technical reports.
%

% Title

% Your title must be in mixed case, not sentence case.
% That means all verbs (including short verbs like be, is, using,and go),
% nouns, adverbs, adjectives should be capitalized, including both words in hyphenated terms, while
% articles, conjunctions, and prepositions are lower case unless they
% directly follow a colon or long dash
\title{Supplementary Material for Exploiting Facial Relationships and Feature Aggregation for Multi-Face Forgery Detection}
\author{
    %Authors
    % All authors must be in the same font size and format.
    Written by AAAI Press Staff\textsuperscript{\rm 1}\thanks{With help from the AAAI Publications Committee.}\\
    AAAI Style Contributions by Pater Patel Schneider,
    Sunil Issar,\\
    J. Scott Penberthy,
    George Ferguson,
    Hans Guesgen,
    Francisco Cruz\equalcontrib,
    Marc Pujol-Gonzalez\equalcontrib
}
\affiliations{
    %Afiliations
    \textsuperscript{\rm 1}Association for the Advancement of Artificial Intelligence\\
    % If you have multiple authors and multiple affiliations
    % use superscripts in text and roman font to identify them.
    % For example,

    % Sunil Issar\textsuperscript{\rm 2},
    % J. Scott Penberthy\textsuperscript{\rm 3},
    % George Ferguson\textsuperscript{\rm 4},
    % Hans Guesgen\textsuperscript{\rm 5}
    % Note that the comma should be placed after the superscript

    1900 Embarcadero Road, Suite 101\\
    Palo Alto, California 94303-3310 USA\\
    % email address must be in roman text type, not monospace or sans serif
    proceedings-questions@aaai.org
%
% See more examples next
}

%Example, Single Author, ->> remove \iffalse,\fi and place them surrounding AAAI title to use it
\iffalse
\title{My Publication Title --- Single Author}
\author {
    Author Name
}
\affiliations{
    Affiliation\\
    Affiliation Line 2\\
    name@example.com
}
\fi

\iffalse
%Example, Multiple Authors, ->> remove \iffalse,\fi and place them surrounding AAAI title to use it
\title{Supplementary Material for Exploiting Facial Relationships and Feature Aggregation \\for Multi-Face Forgery Detection}
\author {
    % Authors
    First Author Name\textsuperscript{\rm 1},
    Second Author Name\textsuperscript{\rm 2},
    Third Author Name\textsuperscript{\rm 1}
}
\affiliations {
    % Affiliations
    \textsuperscript{\rm 1}Affiliation 1\\
    \textsuperscript{\rm 2}Affiliation 2\\
    firstAuthor@affiliation1.com, secondAuthor@affilation2.com, thirdAuthor@affiliation1.com
}
\fi

% REMOVE THIS: bibentry
% This is only needed to show inline citations in the guidelines document. You should not need it and can safely delete it.
\usepackage{bibentry}
% END REMOVE bibentry

% \begin{document}

\maketitle

% \begin{abstract}
%  Face forgery techniques have emerged as a forefront concern, and numerous detection approaches have been proposed to address this challenge. However, existing methods predominantly concentrate on single-face manipulation detection, leaving the more intricate and realistic realm of multi-face forgeries relatively unexplored. This paper proposes a novel framework explicitly tailored for multi-face forgery detection,
%  % called DEAR 
%  %that is specifically designed to detect multi-face forgery, 
%  filling a critical gap in the current research. The framework mainly involves two modules: (i) a facial relationships learning module, which generates distinguishable local features for each face within images,
%  % the similarity and difference relationships between different faces in each multi-face image, 
%  (ii) a global feature aggregation module that leverages the mutual constraints between global and local information to enhance forgery detection accuracy. 
%  % In addition, we xxx to enhance xxx.
%  Our experimental results on two publicly available multi-face forgery datasets demonstrate that the proposed approach achieves state-of-the-art performance in multi-face forgery detection scenarios. 
%  % Moreover, our framework can be seamlessly integrated into existing detection methods to enhance performance.  
% \end{abstract}

\section{Selection of Loss Weights}
In section 3.4 in the main text, we have defined the total loss as follows:
\begin{equation}
    \mathcal L = \mathcal L_{global} + \lambda_1 \mathcal L_{local} + \lambda_2 \mathcal L_{pull} + \lambda_3 \mathcal L_{push}.
\end{equation}
In this formulation, the values we have specifically chosen for the weighting coefficients $\lambda_1$, $\lambda_2$, and $\lambda_3$ are set at 1, 4, and 1, respectively. This strategic assignment of coefficients achieves a balanced emphasis on each loss component, ensuring that no single loss term dominates the training process.  Empirical validation substantiates that this equilibrium contributes significantly to the model's convergence efficiency and overall effectiveness.

\section{Evolution of the Self-similarity Matrix}
In order to gain deeper insights into how the self-similarity matrix evolves during the course of model training, we employed a visualization approach to track its changes. Figure 1 provides a visual representation of the matrix's dynamic behavior. As we can see that at the initial stages of model training, there is a notable absence of strong correlations among the various features encapsulated within the similarity matrix. However, as the training iterations progress, a remarkable transformation occurs within the similarity matrix. Specifically, the facial features belonging to the same class gradually begin to exhibit discernible patterns of correlation, indicating the emergence of underlying relationships. This evolving pattern of correlation continues to intensify as the model undergoes successive training rounds.

These findings serve as compelling evidence of the success of our model in capturing and learning intrinsic relationships between facial features. The progressive increase in correlation among same-class facial attributes throughout the training validates the model's capacity to discern subtle distinctions and interdependencies among faces. Consequently, it can be inferred that the model not only recognizes individual facial attributes but also comprehends the broader context of facial representation. It demonstrates that the proposed self-similarity matrix facilitates the model's capability to establish meaningful connections between faces, contributing to its enhanced performance in multi-face detection task.

\begin{figure*}[t]
  \centering
  \begin{subfigure}[b]{0.33\textwidth}
    \includegraphics[width=\textwidth]{AnonymousSubmission/LaTeX/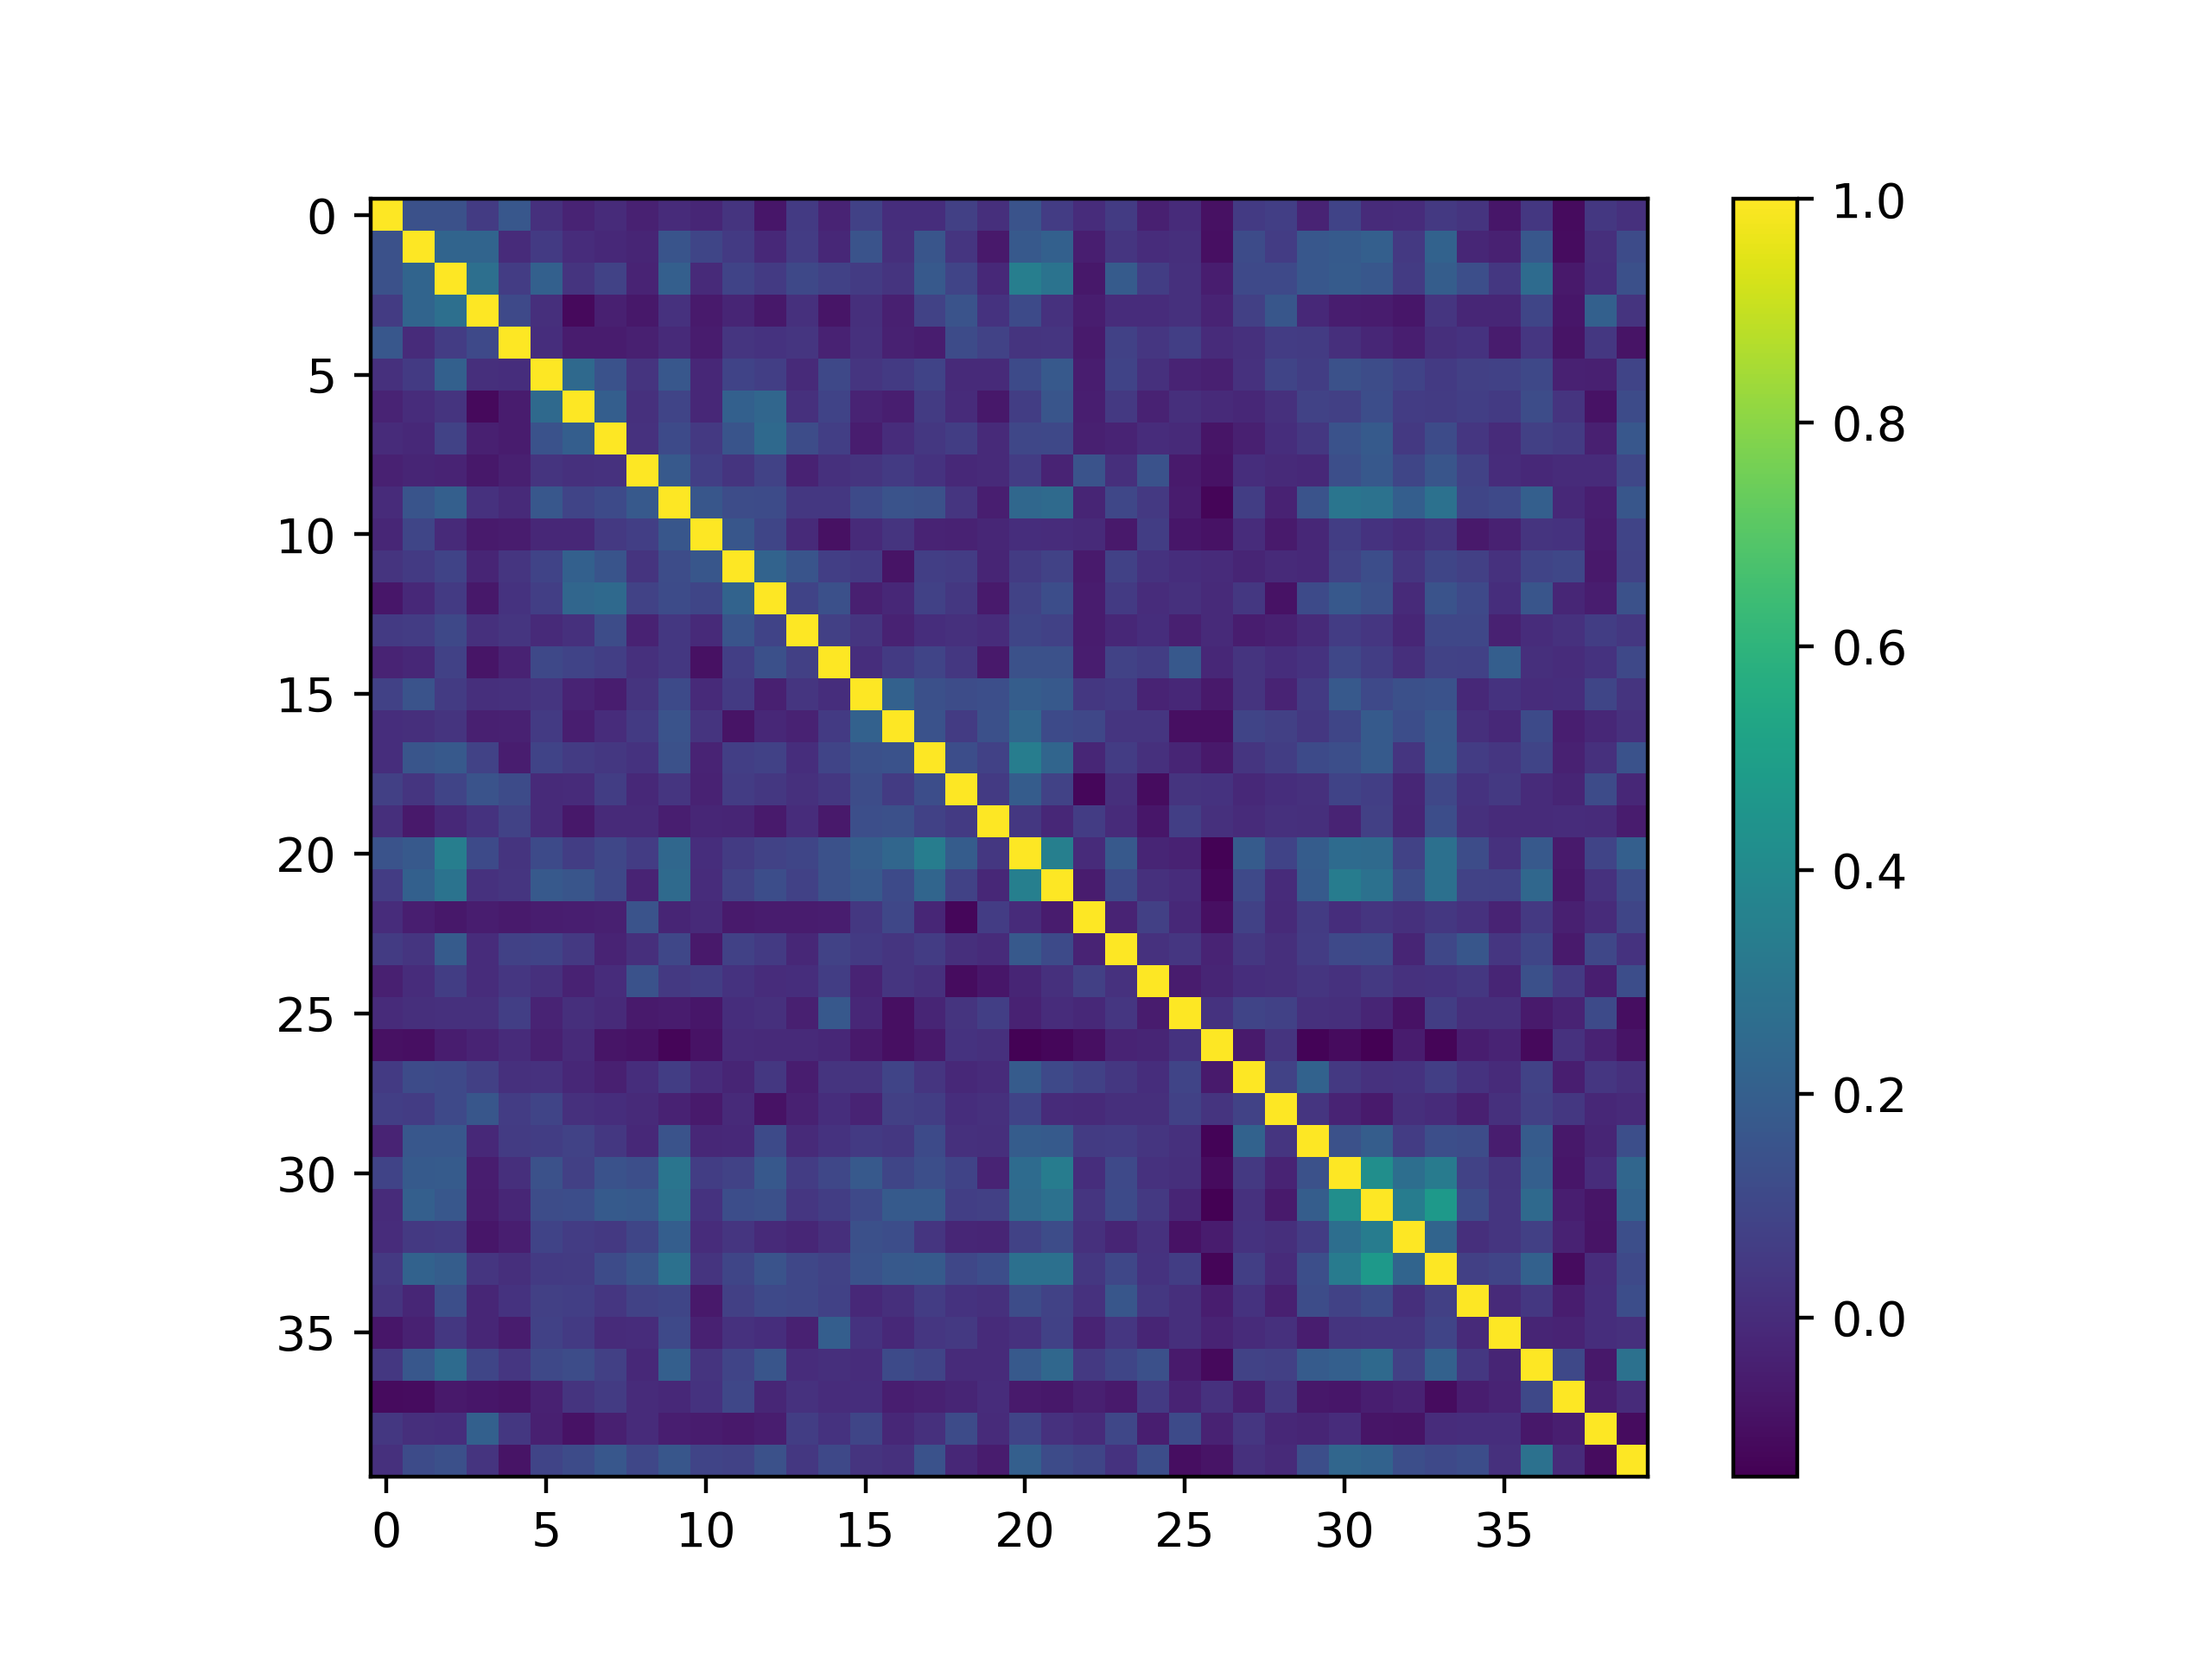}
    \label{fig:sub1}
    \caption{epoch 1}
  \end{subfigure}
  \begin{subfigure}[b]{0.33\textwidth}
    \includegraphics[width=\textwidth]{AnonymousSubmission/LaTeX/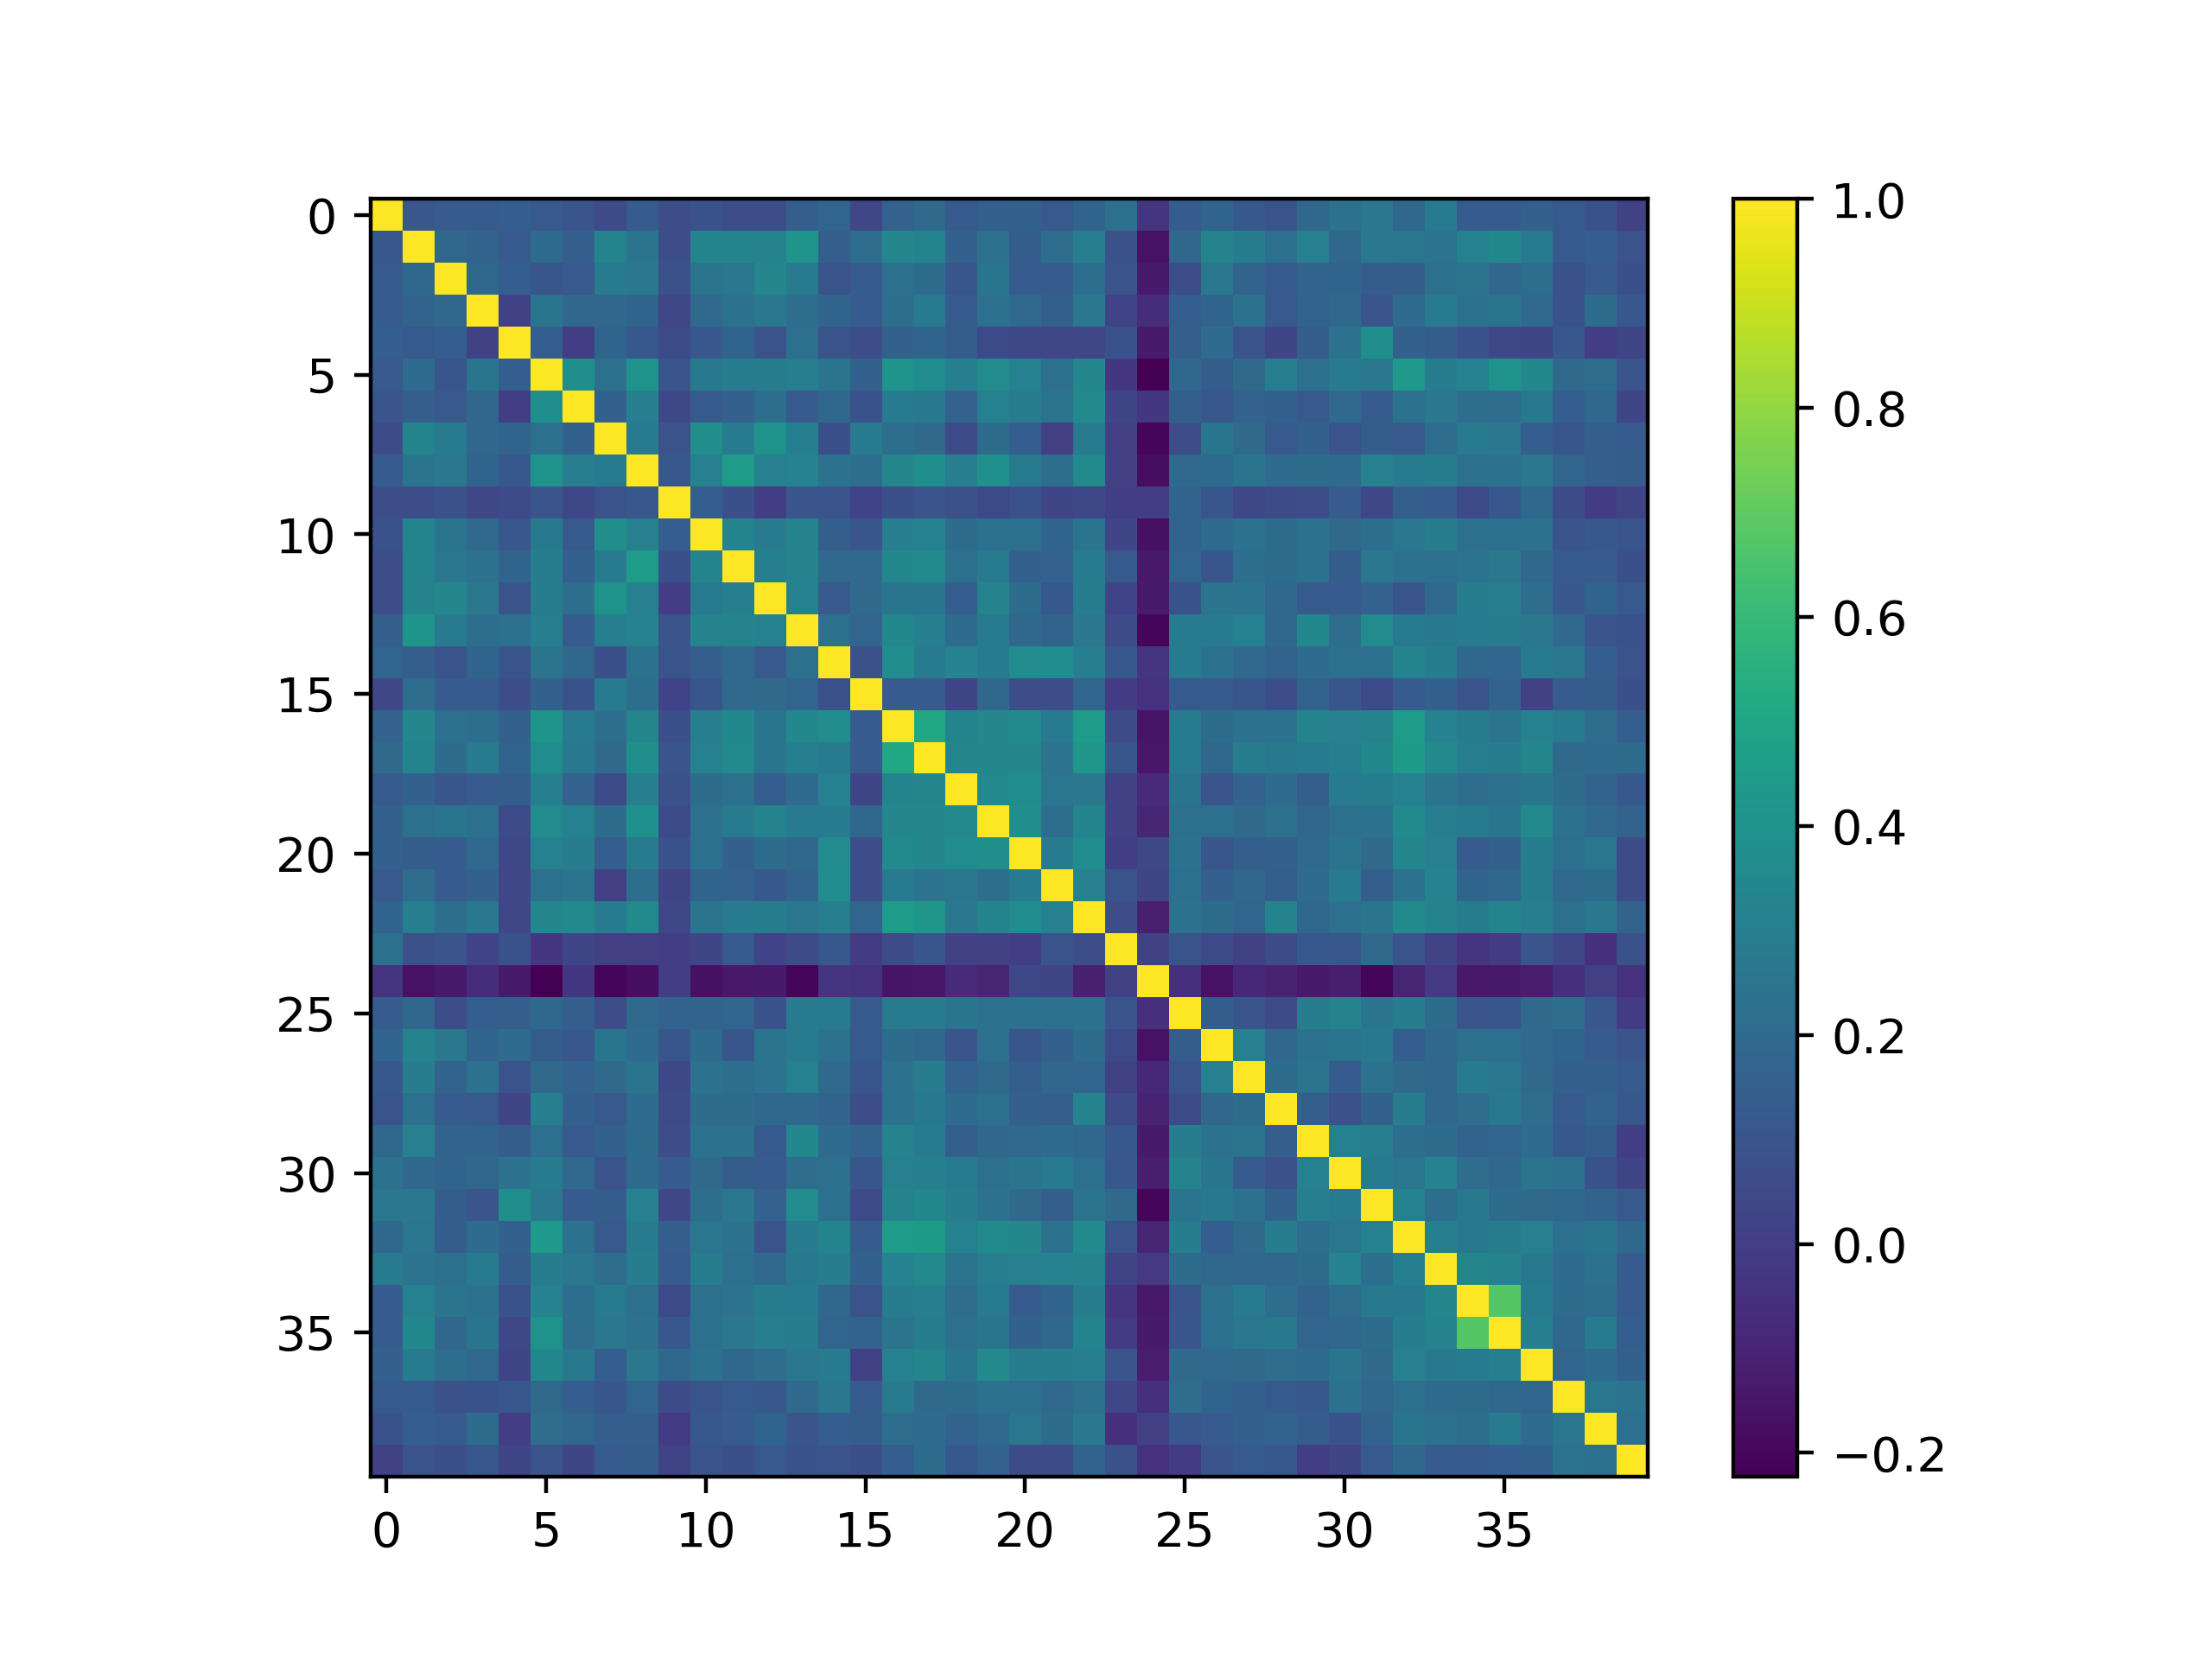}
    \label{fig:sub2}
    \caption{epoch 2}
  \end{subfigure}
  \begin{subfigure}[b]{0.33\textwidth}
    \includegraphics[width=\textwidth]{AnonymousSubmission/LaTeX/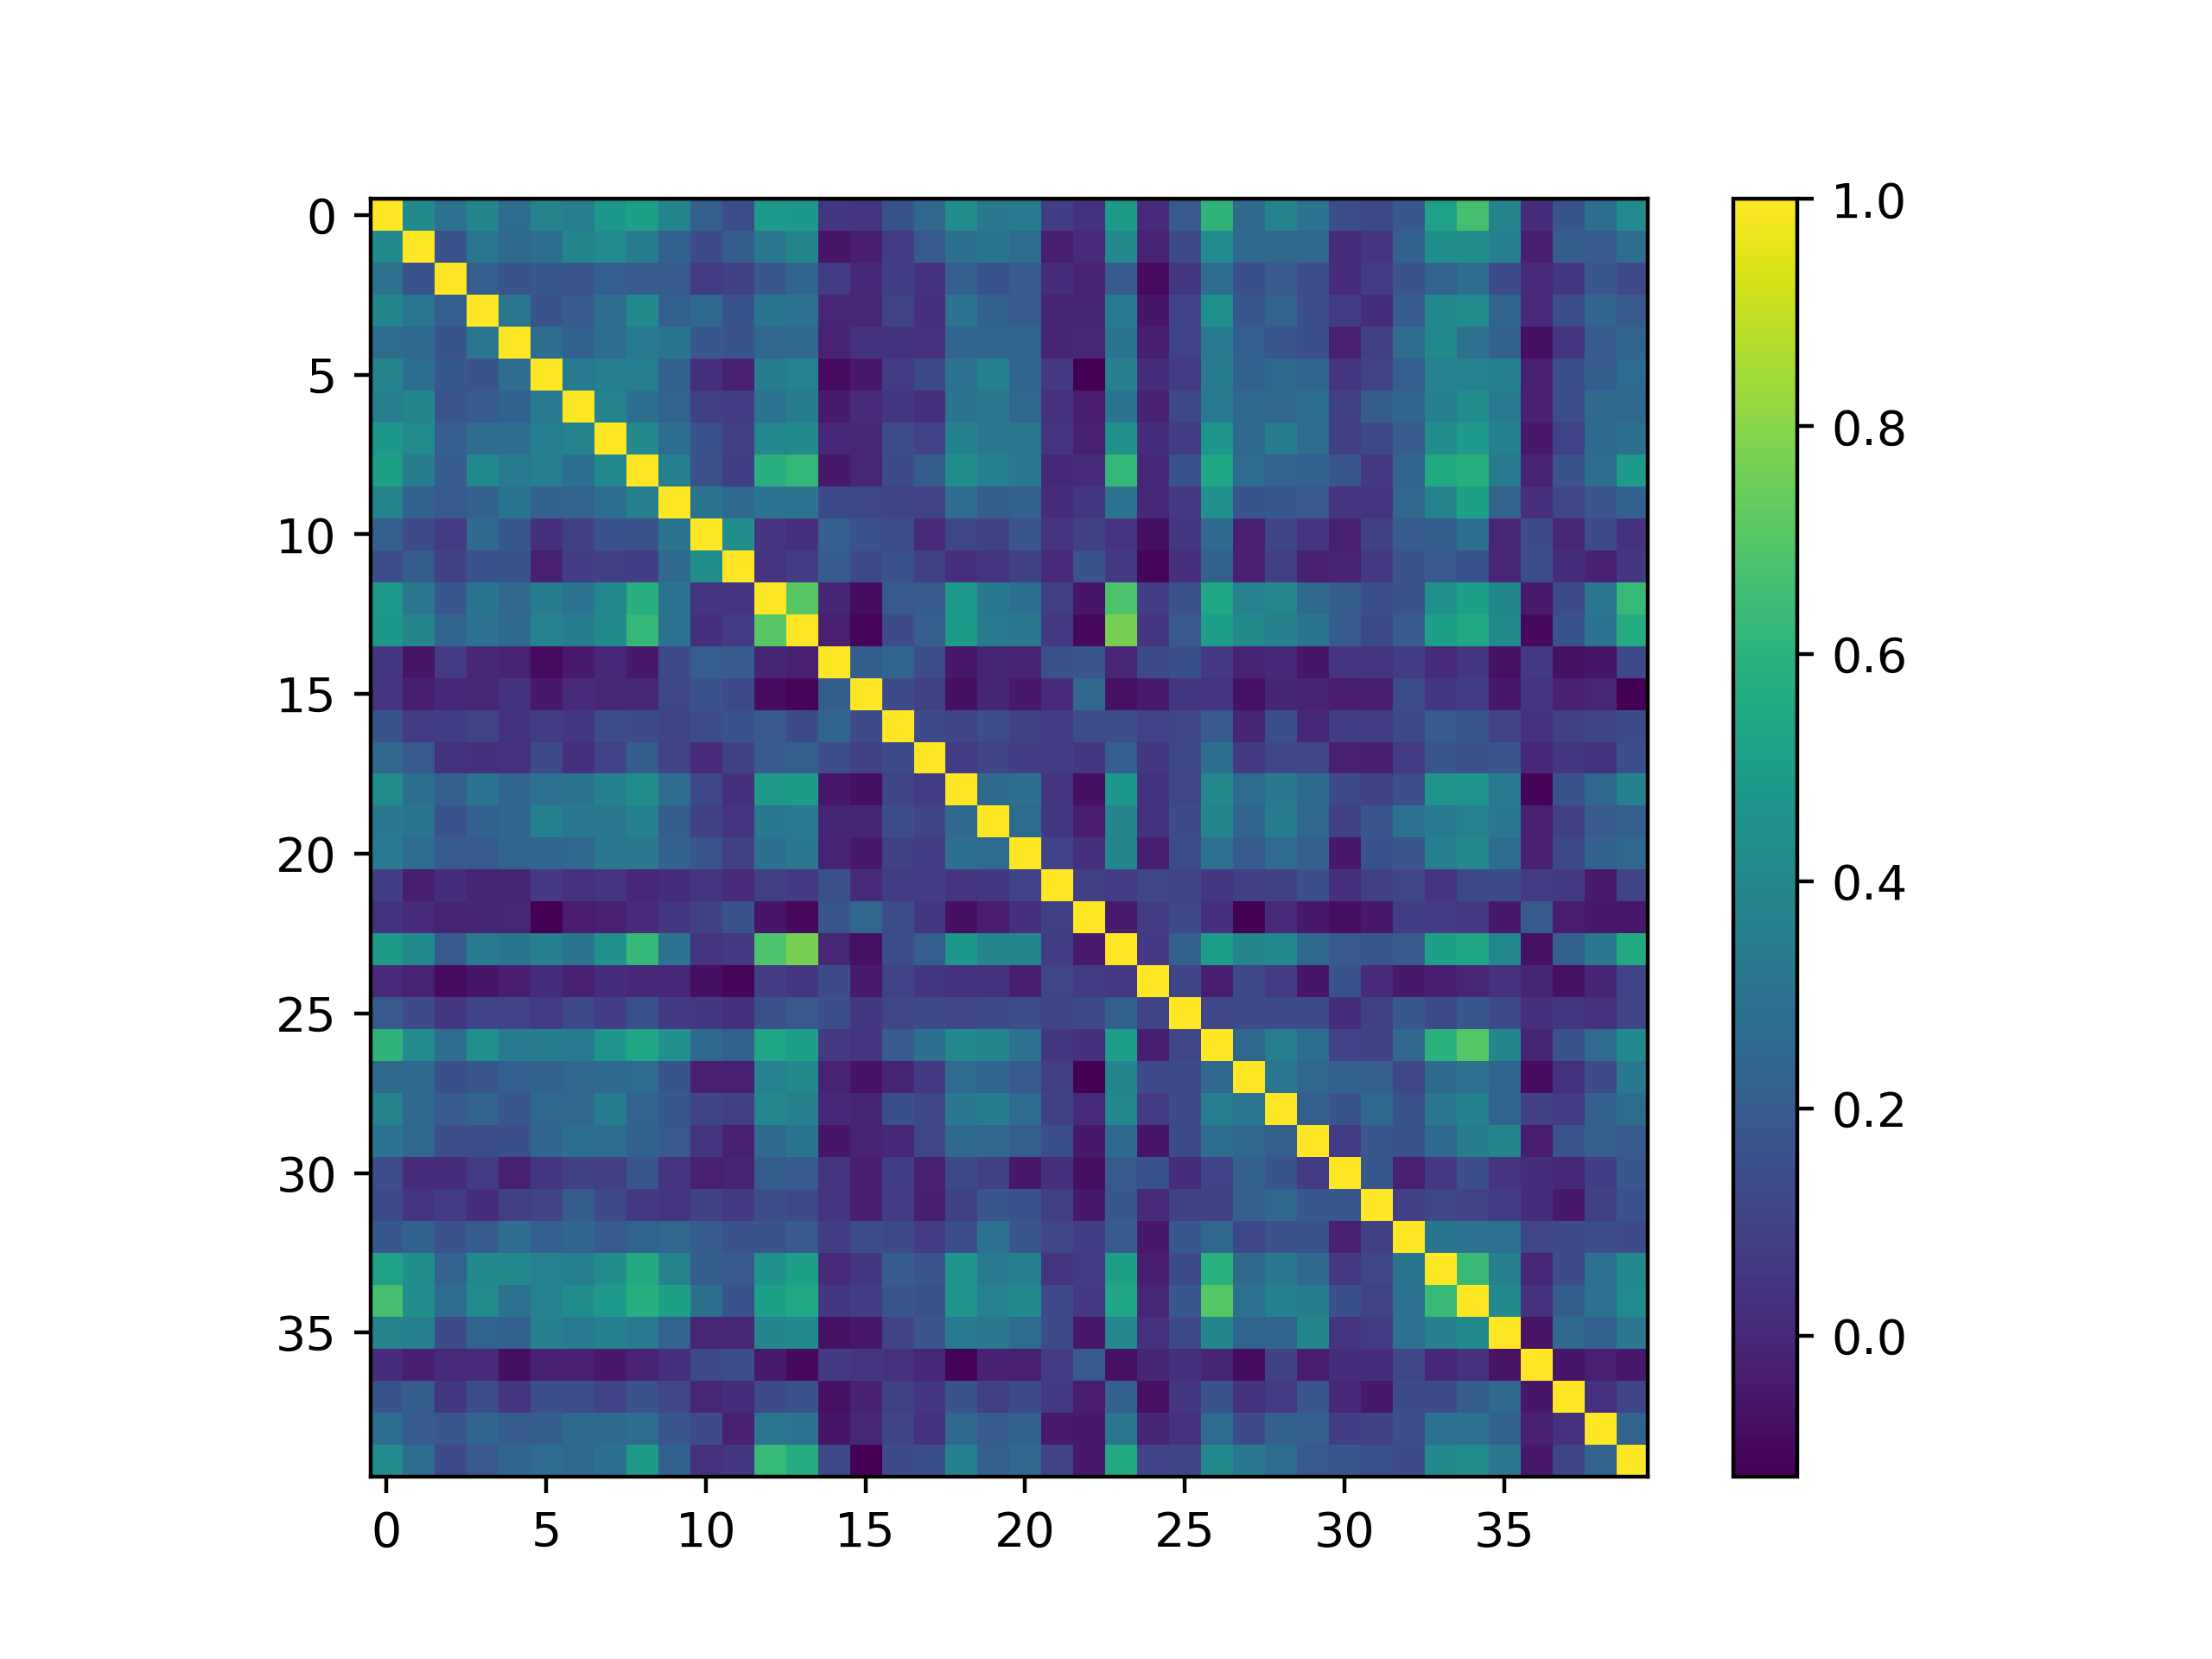}
    \label{fig:sub3}
    \caption{epoch 3}
  \end{subfigure}

  \begin{subfigure}[b]{0.33\textwidth}
    \includegraphics[width=\textwidth]{AnonymousSubmission/LaTeX/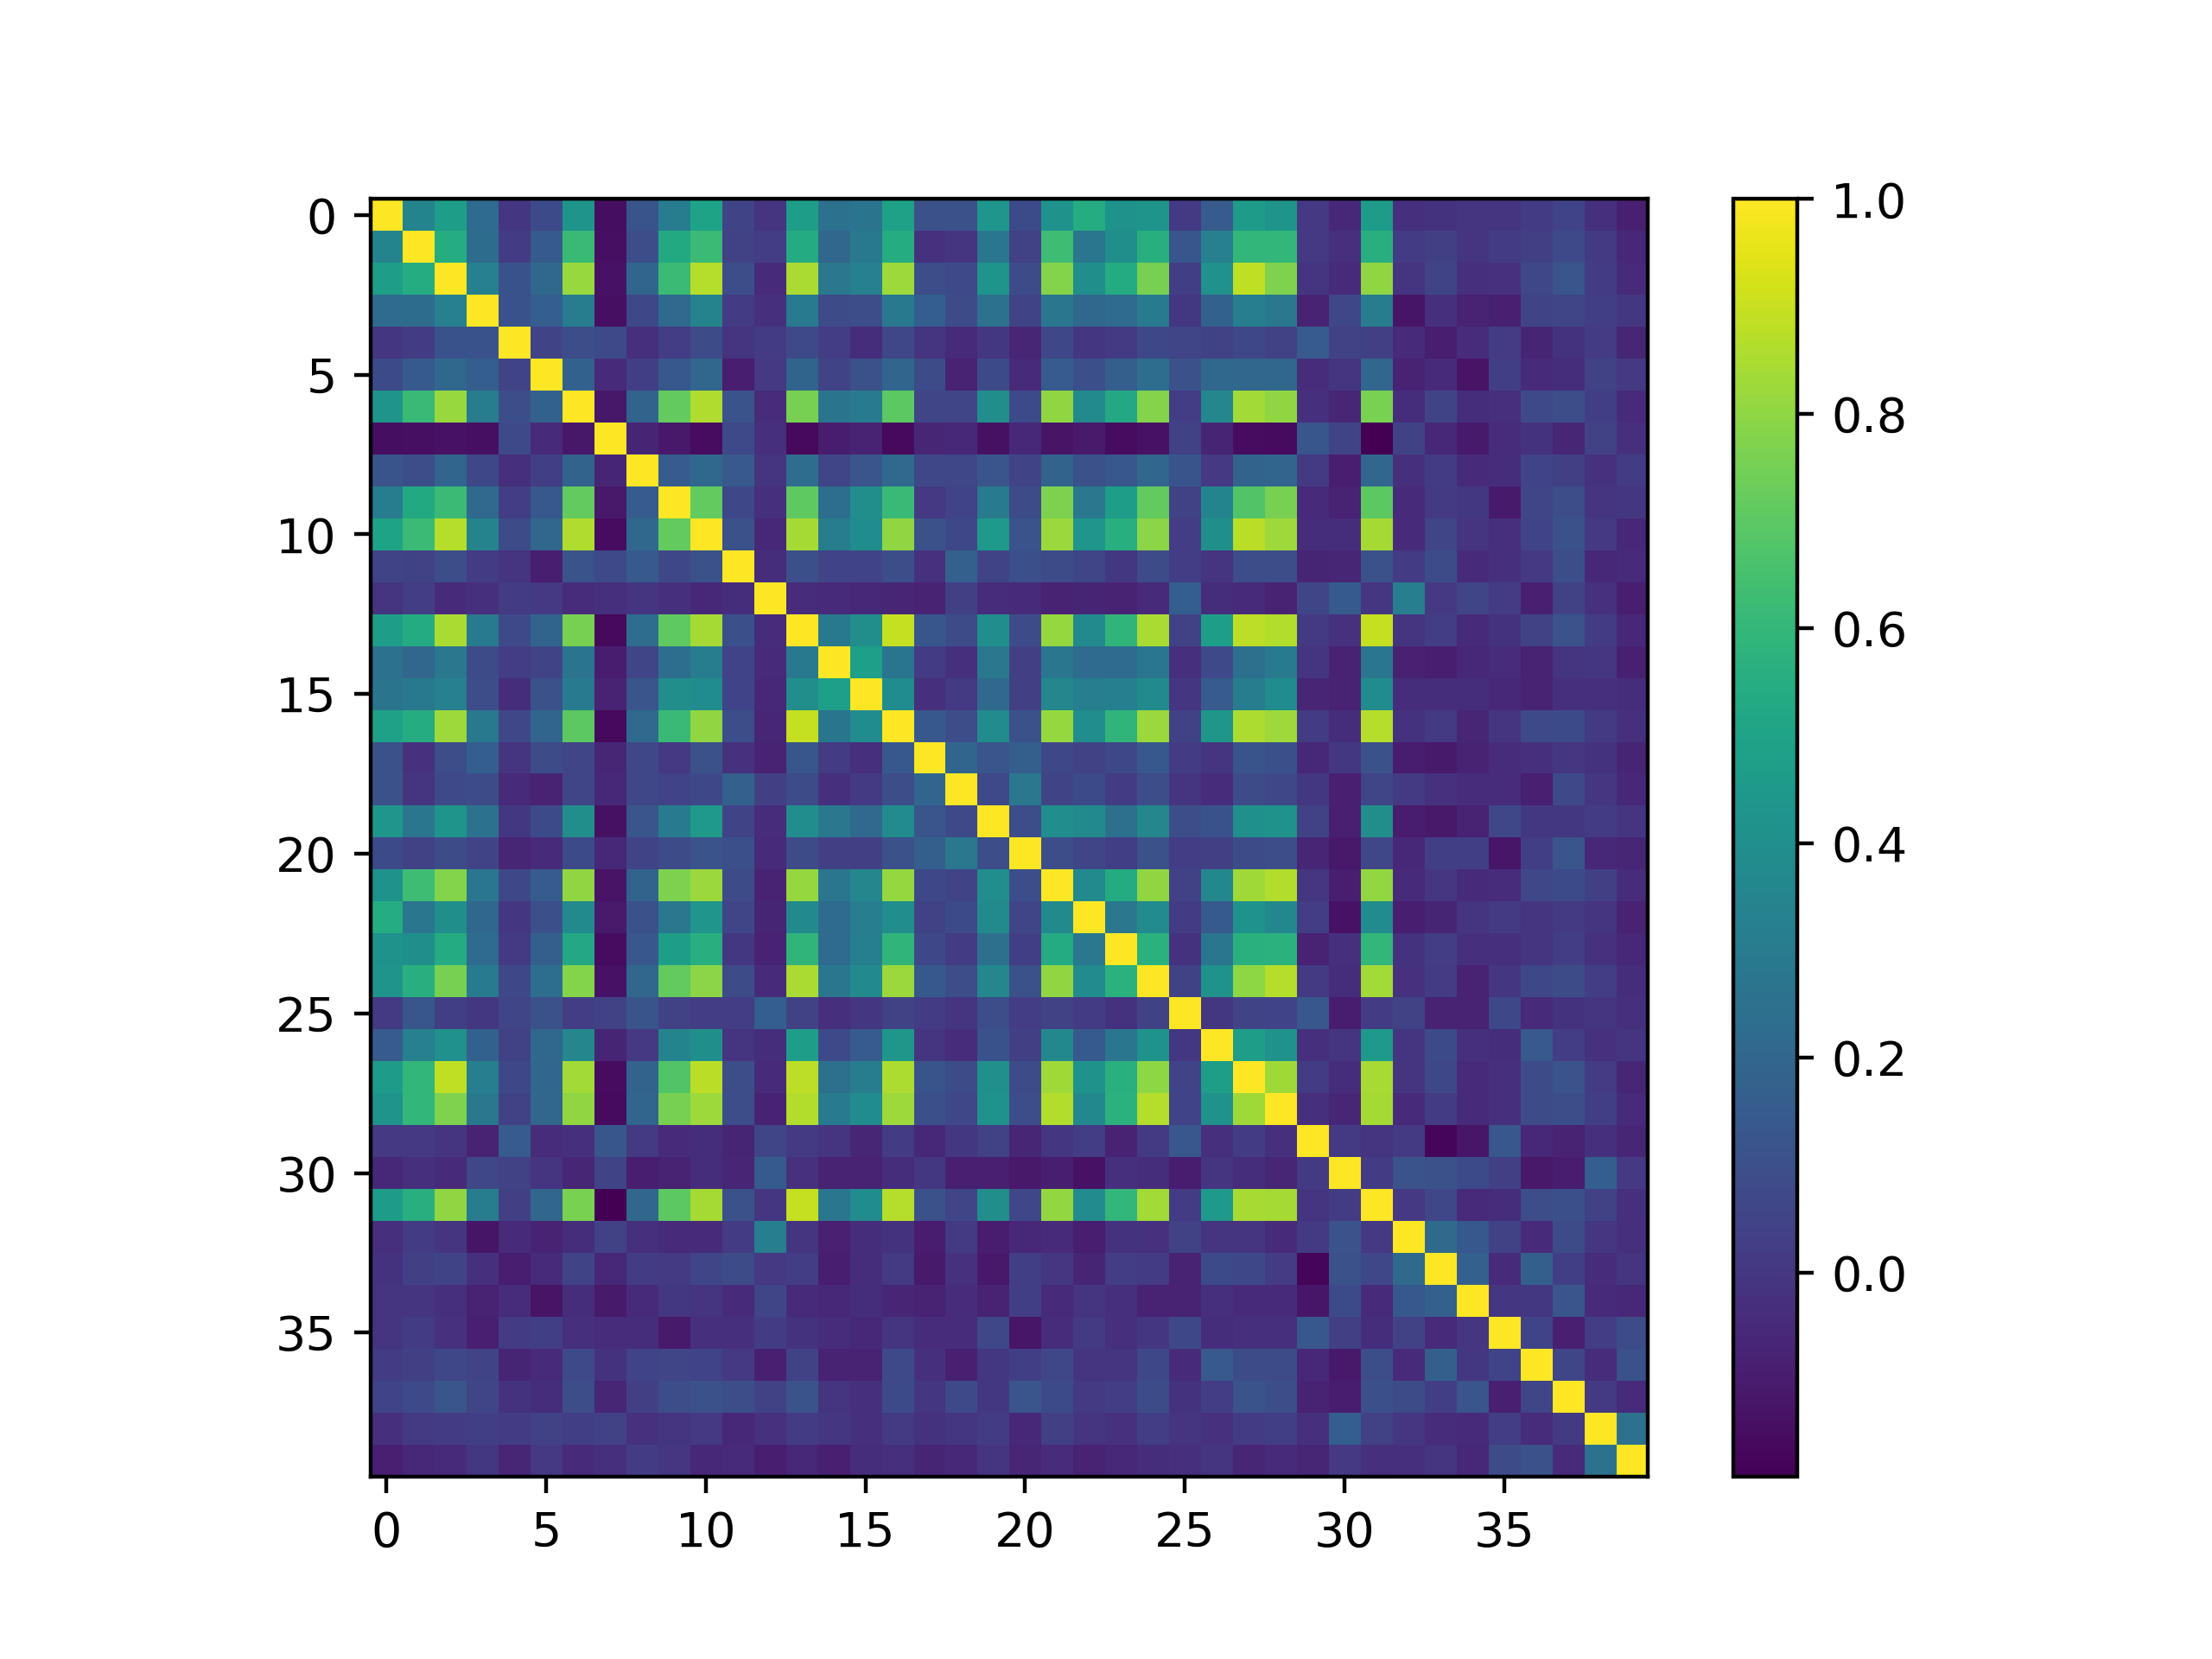}
    \label{fig:sub4}
    \caption{epoch 4}
  \end{subfigure}
  \begin{subfigure}[b]{0.33\textwidth}
    \includegraphics[width=\textwidth]{AnonymousSubmission/LaTeX/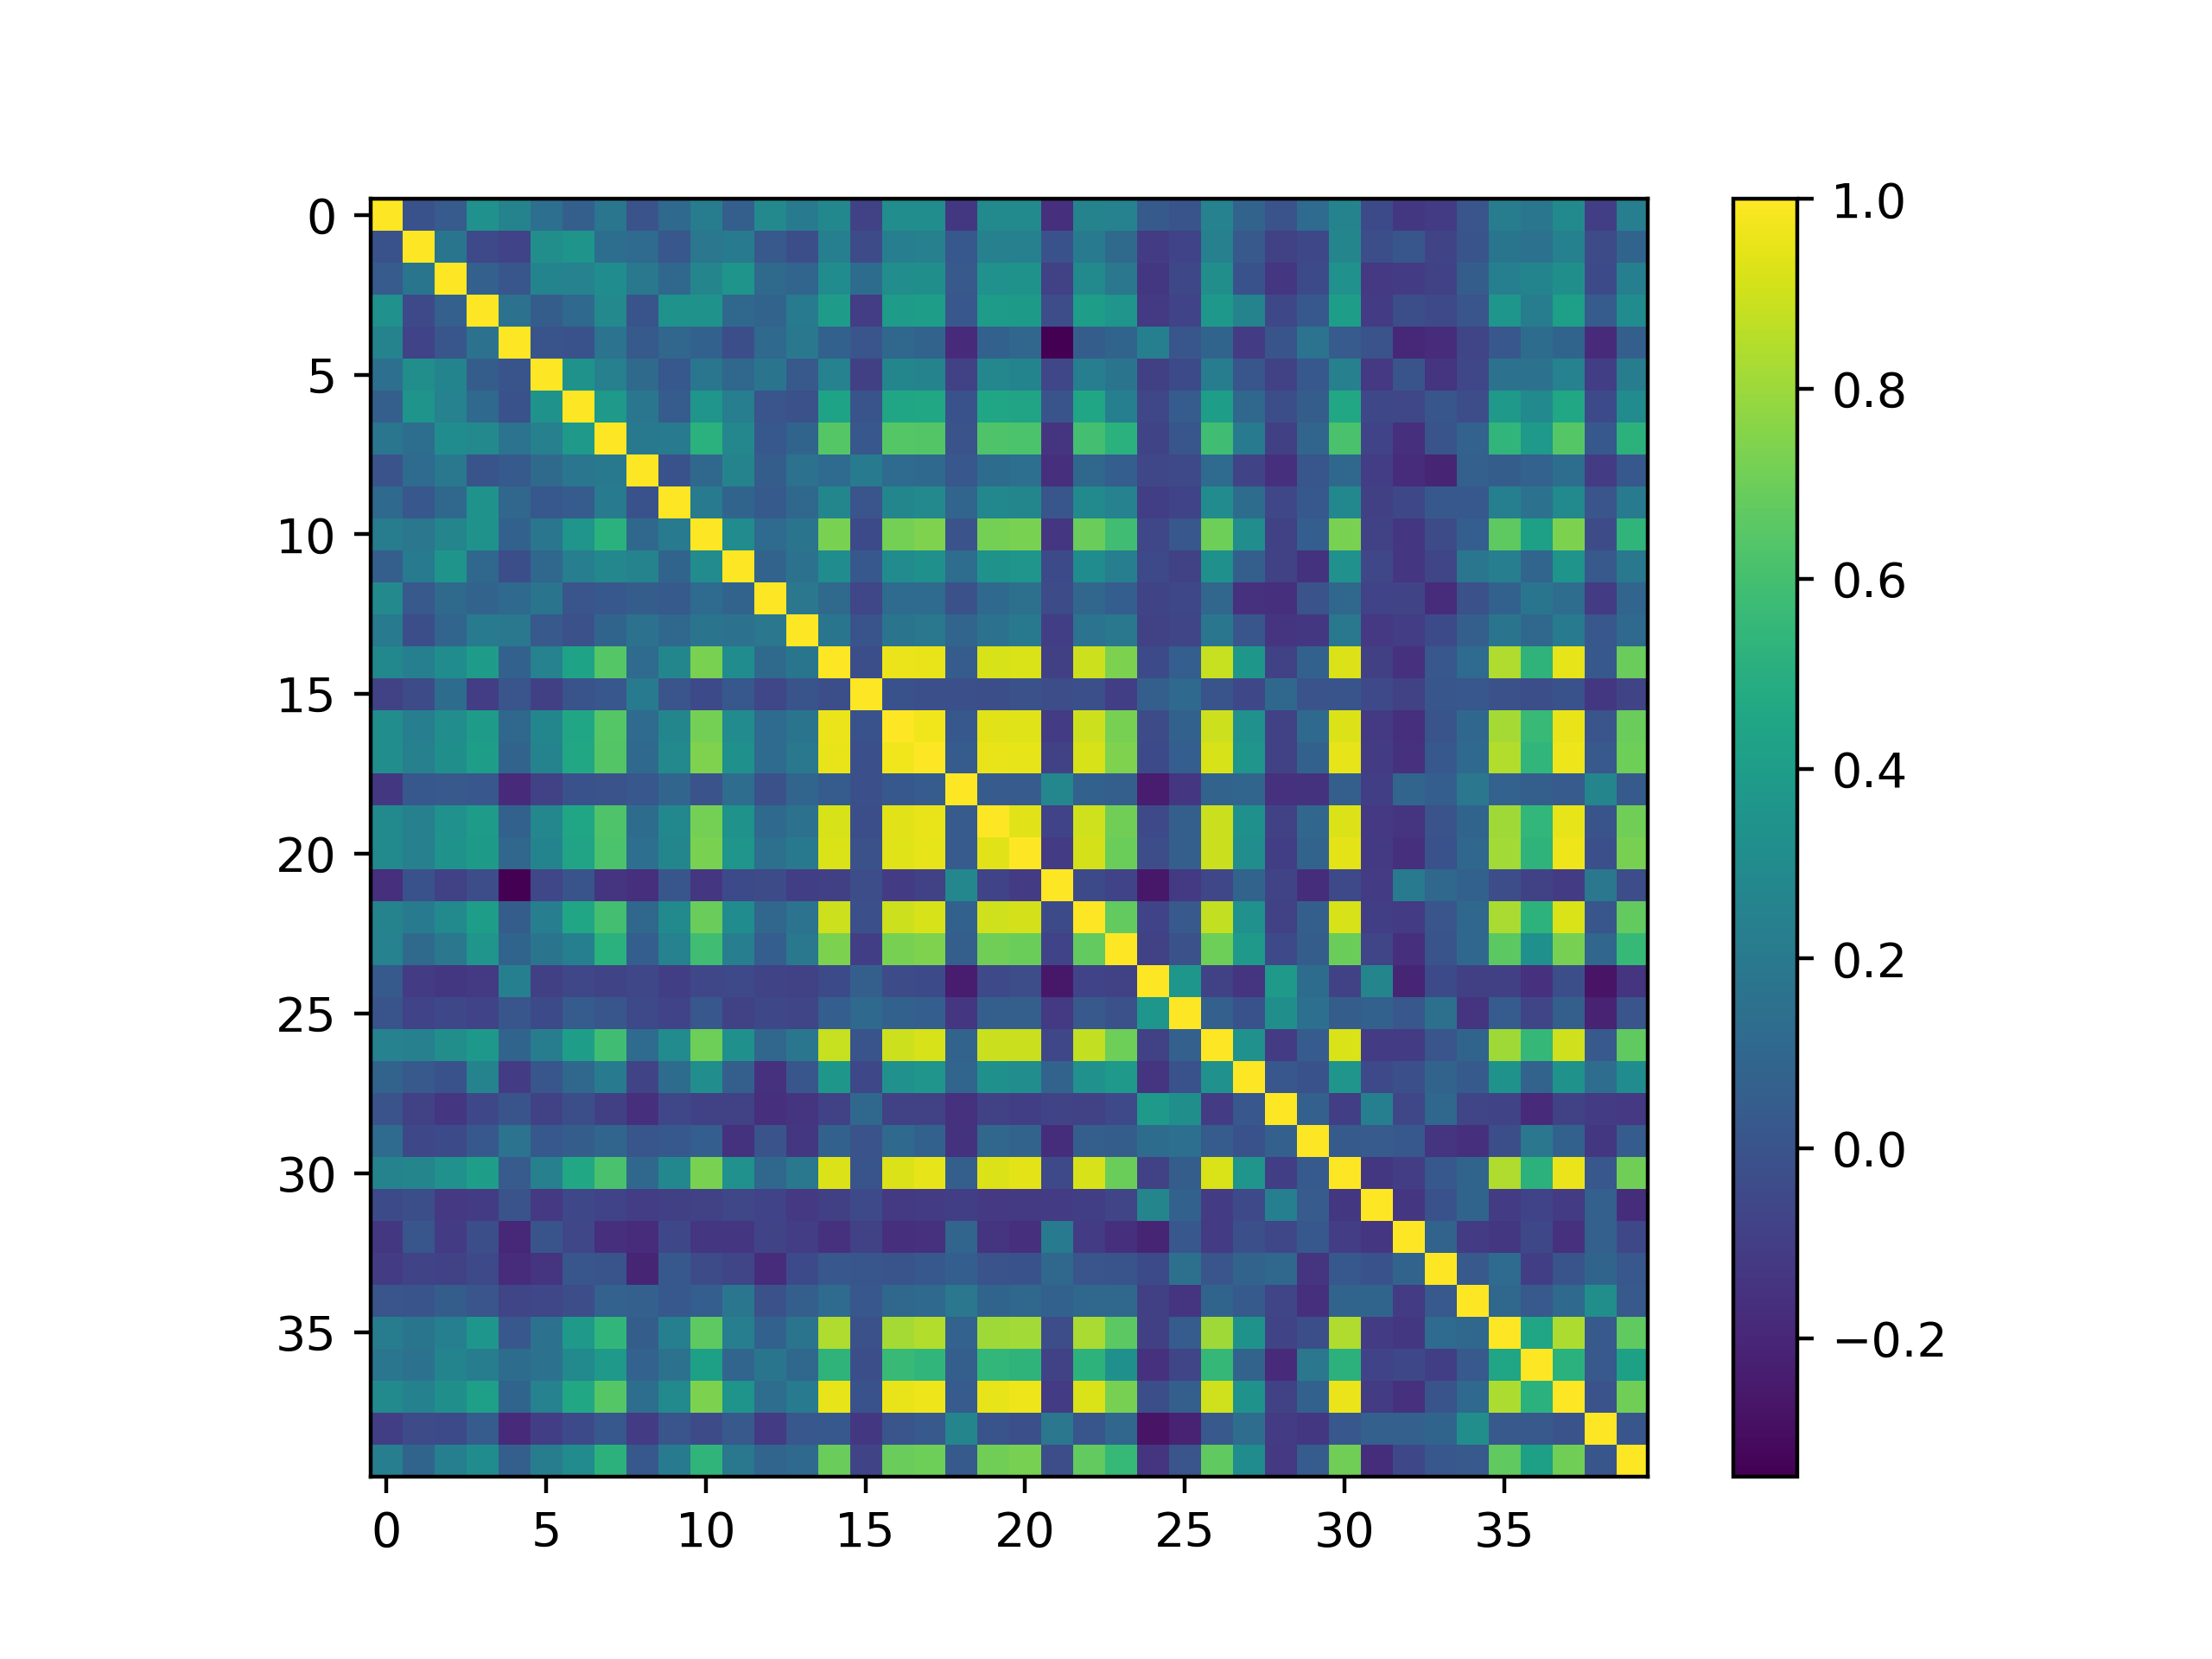}
    \label{fig:sub5}
    \caption{epoch 7}
  \end{subfigure}
  \begin{subfigure}[b]{0.33\textwidth}
    \includegraphics[width=\textwidth]{AnonymousSubmission/LaTeX/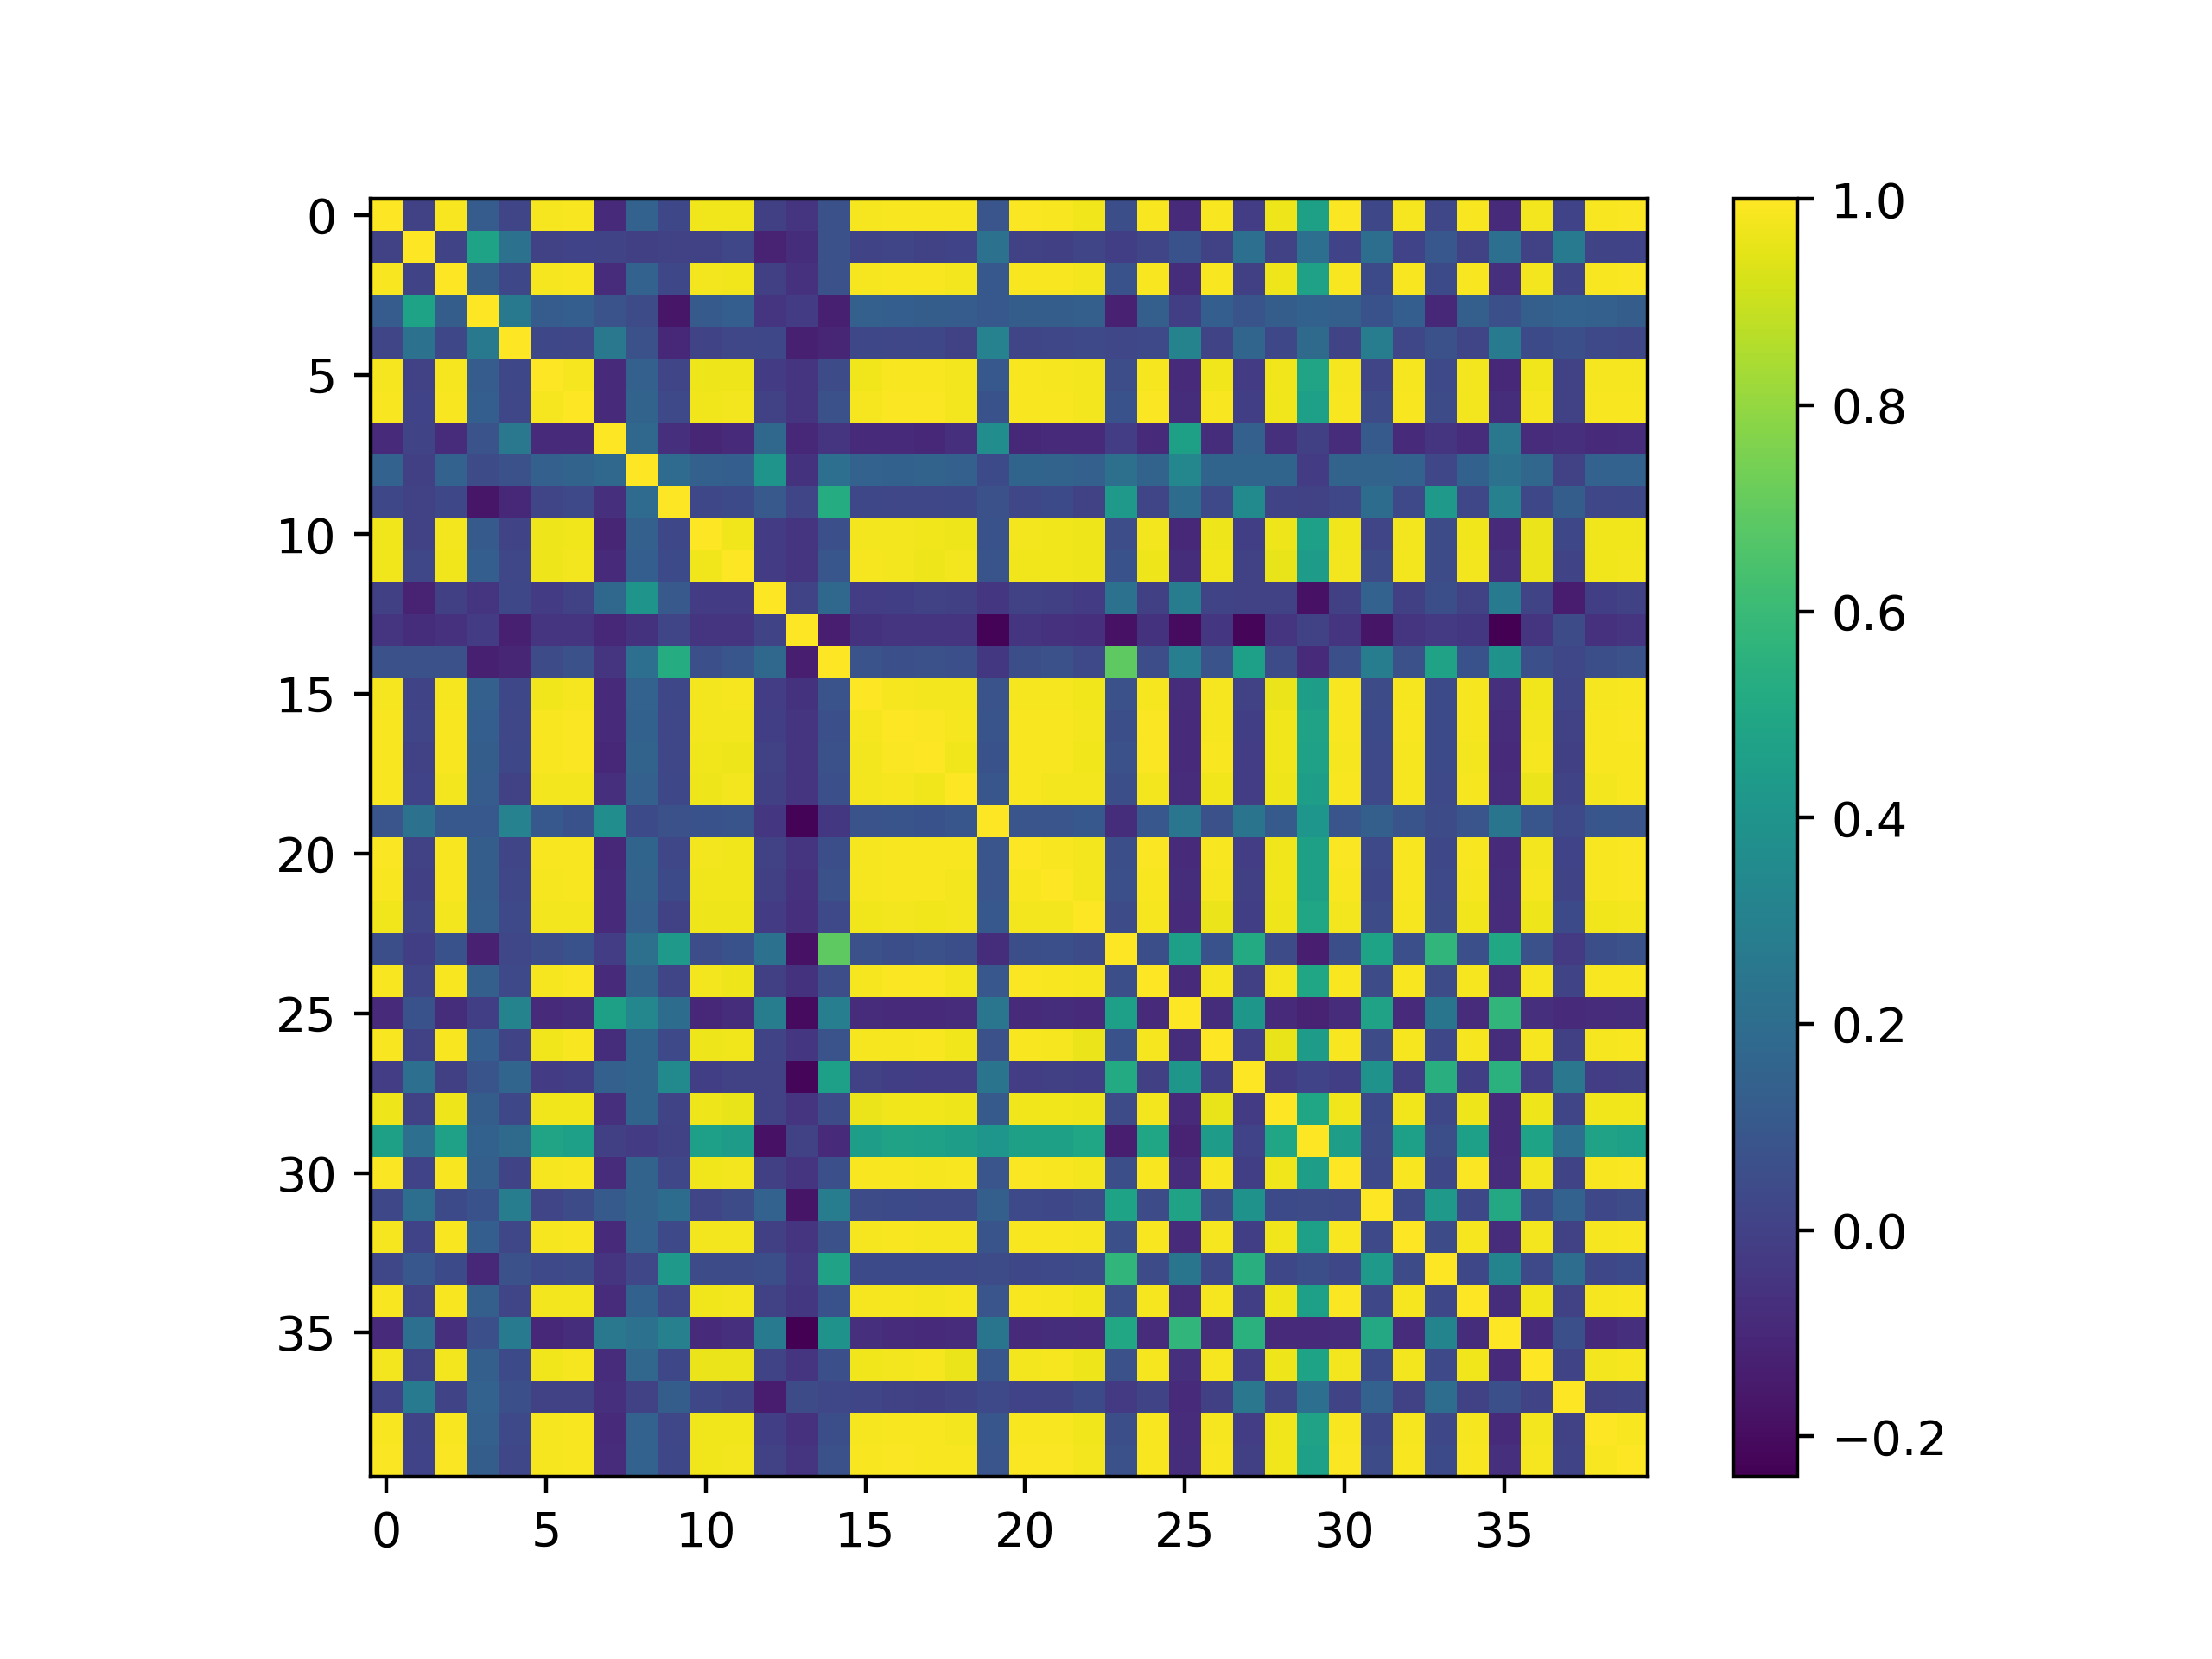}
    \label{fig:sub6}
    \caption{epoch 10}
  \end{subfigure}

  \caption{Trend of Self-similarity Matrix Evolution. With the continuous increase in the number of training iterations, facial features gradually begin to exhibit discernible patterns of correlation.}
  \label{}
\end{figure*}

\end{document}
